# Supplementary material for: Cluster-based multidimensional scaling embedding tool for data visualization
Source: arXiv:2209.06614 ancillary file (2024-05-24)
Supplement: Supplementary file 1 [file Supplementary_information_clMDS.pdf]

# Supplementary Information: Cluster-based Multidimensional Scaling embedding tool for data visualization

**Patricia Hernández-León** PATRICIA.HERNANDEZLEON@AALTO.FI
*Department of Chemistry and Materials Science*
*Aalto University*
*02150, Espoo, Finland*

**Miguel A. Caro** MCAROBA@GMAIL.COM
*Department of Chemistry and Materials Science*
*Aalto University*
*02150, Espoo, Finland*

This document contains miscellaneous information to support the manuscript "Cluster-based Multidimensional Scaling embedding tool for data visualization".

© .

License: CC-BY 4.0, see https://creativecommons.org/licenses/by/4.0/.

## CHO structural database: full comparison of methods

Figures 1 and 2 show the best embeddings obtained for a subset of CHO database (Golze et al., 2022), using different dimensionality reduction methods. They include different hyperparameter estimations for t-SNE and UMAP. We maximized the silhouette score (Rousseeuw, 1987) considering three classifications: (1) chemical species classification; (2) k-medoids clustering performed by cl-MDS, with hierarchy $h = [30, 1]$; and (3) classical chemical configurations, i.e., simple hybridizations and functional groups. The resulting embeddings are shown following the same order in the figures:

| classification | `perplexity` (t-SNE) | `n_neighbours` (UMAP) |
|---|---|---|
| (1) | 50 | 628 |
| (2) | 43 | 62 |
| (3) | 50 | 11 |

Note that we optimized only those hyperparameters that tune the local/global ratio of the visualization. In particular, `perplexity` values set the size of the initial graph preserved by t-SNE, focusing on global information mostly when approaching 50. Similarly, `n_neighbors` parameter sets the size of the initial fuzzy set in UMAP, with the locality fixed by the number of neighbors. While t-SNE only favours global visualizations for this sample, UMAP offers a much interesting range of embeddings (see Fig. 2). Here we can see the limits of the `n_neighbors` hyperparameter, compare to the `hierarchy` of cl-MDS: each row with UMAP embeddings has an optimal visualization for its corresponding classification, but the display of the other "layers" of locality is worsened. In practice, three different visualizations are needed to capture all the information, instead of one.

### References

D. Golze, M. Hirvensalo, P. Hernández-León, A. Aarva, J. Etula, T. Susi, P. Rinke, T. Laurila, and M. A. Caro. Accurate computational prediction of core-electron binding energies in carbon-based materials: A machine-learning model combining density-functional theory and gw. *Chemistry of Materials*, 34(14):6240–6254, 2022.

P. J. Rousseeuw. Silhouettes: A graphical aid to the interpretation and validation of cluster analysis. *Journal of Computational and Applied Mathematics*, 20:53–65, 1987.

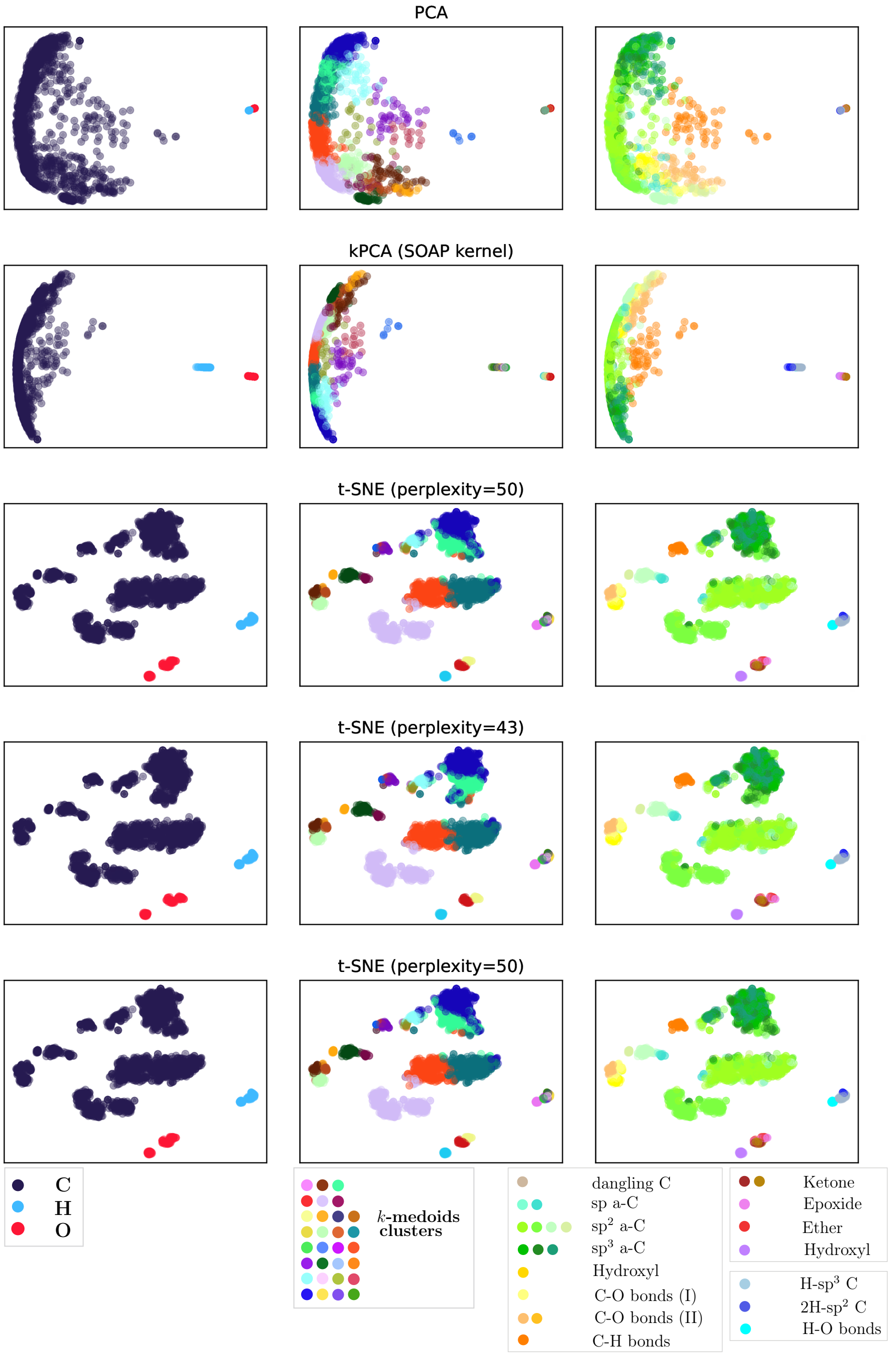


Figure 1: Embedding of 2000 data points from the CHO database using different methods (part 1). Each column is coloured according to (1) chemical species (C, H, O), (2) k-medoids clustering $h = [30, 1]$, and (3) motifs classification.

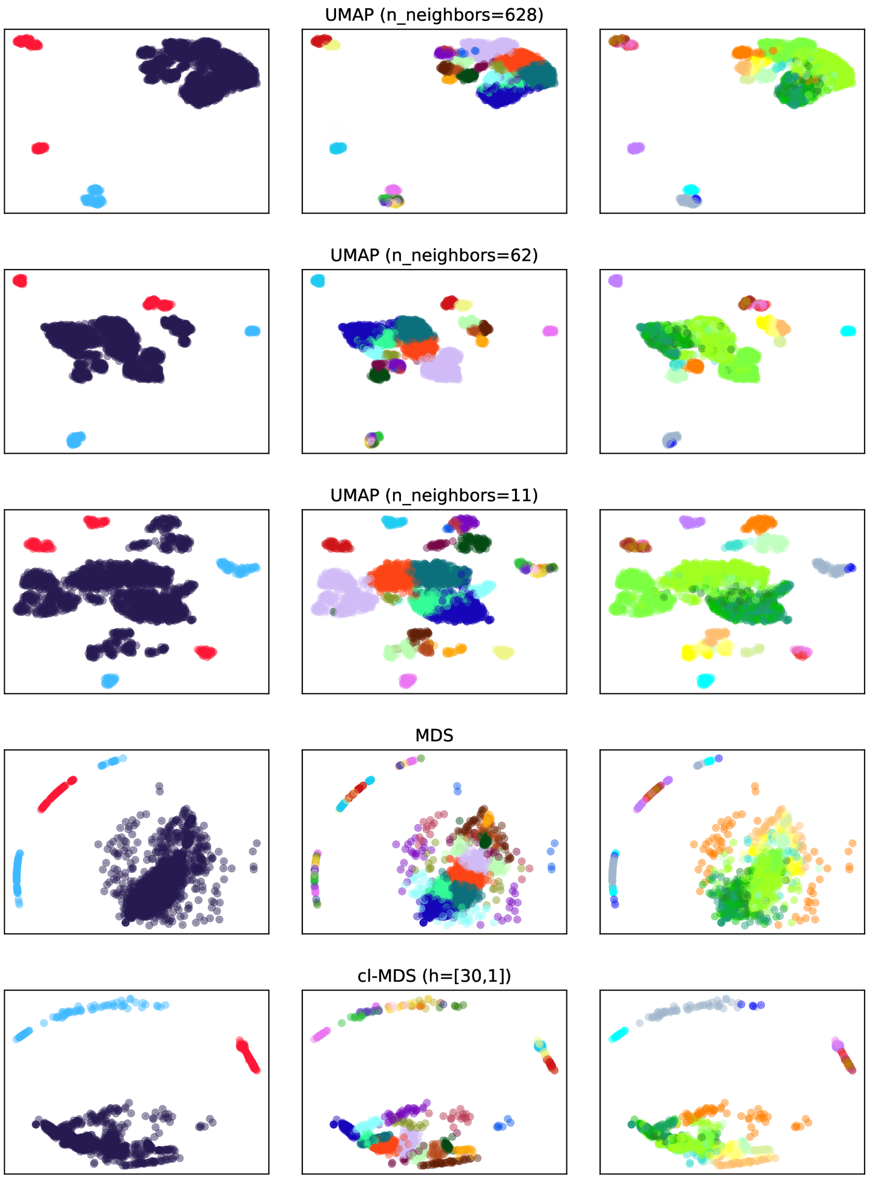


Figure 2: Embedding of 2000 data points from the CHO database using different methods (part 2). Each column is coloured according to (1) chemical species (C, H, O), (2) k-medoids clustering $h = [30, 1]$, and (3) motifs classification. Check the legend in Fig. 1.
